# Supplementary material for: Activated lone-pair electrons lead to low lattice thermal conductivity: a case study of boron arsenide
Source: arXiv:1904.00329 source file (2019-03-31)
Supplement: Supplementary file 1 [file SI.pdf]

Supplementary Information for

# Activated lone-pair electrons lead to low lattice thermal conductivity: a case study of boron arsenide


Guangzhao Qin,[1,2*] Zhenzhen Qin,[3] Huimin Wang,[4,2] and Ming Hu[2†]

[1]*Institute of Mineral Engineering, Division of Materials Science and Engineering, Faculty of Georesources and Materials Engineering, RWTH Aachen University, Aachen 52064, Germany*

[2]*Department of Mechanical Engineering, University of South Carolina, Columbia, SC 29208, USA*

[3]*International Laboratory for Quantum Functional Materials of Henan, and School of Physics and Engineering, Zhengzhou University, Zhengzhou 450001, China*

[4]*College of Engineering and Applied Science, Nanjing University, Nanjing 210023, China*



[*] Author to whom correspondence should be addressed. G. Qin, E-Mail: qin.phys@gmail.com

[†] Author to whom correspondence should be addressed. M. Hu, E-Mail: hu@sc.edu

**Supplemental Table 1.** The thermal conductivity of typical systems in the 3D (*diamond-like cubic*) and 2D (*graphene-like honeycomb*) forms. All the thermal conductivity of the systems in the 3D form are from Refs. [*Phys. Rev. Lett.* **111,** 025901 (2013), *Phys. Rev. B* **87,** 165201 (2013)]. The thermal conductivity of the systems in the 2D form (graphene, silicene, BN, AlN, GaN) are partially from previous reports in Refs. [*Nano Energy* **50,** 425-430 (2018), *Nanoscale* **9,** 7227-7234 (2017)] and partially from the calculations in this study (BSb, BAs, BP, SiC). As for the calculations in this study, all the calculation procedures follow that of BAs with full test of the parameters as stated in the section of computational details in the main text.

| | Thermal conductivity (W/mK) | | Electronegativity difference | Mass ratio |
|---|---|---|---|---|
| | 3D form | 2D form | | |
| C | 2290 | 3094.98 | 0 | 1 |
| Si | 145 | 19.21 (*buckled*) | 0 | 1 |
| BN | 940 | 245.45 | 1 | 0.77184 |
| AlN | 319 | 74.43 | 1.43 | 0.51912 |
| GaN | 253 | 14.93 | 1.23 | 0.20089 |
| BP | 580 | 22.5 | 0.15 | 0.34904 |
| BAs | 2240 (3-*phonons*) | 137.7 | 0.14 | 0.1443 |
| BSb | 465 | 21.9 | 0.01 | 0.08879 |
| SiC | 490 | 81.9 | 0.65 | 0.42766 |

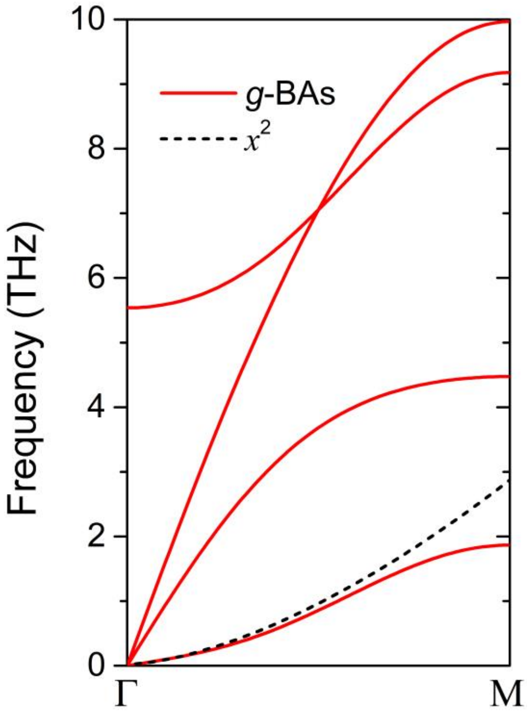


**Supplemental Figure 1.** The phonon dispersion of acoustic phonon branches of *g*-BAs along the high-symmetry points (Γ-M), where the black dash line shows the quadratic behavior of *z*-direction flexural acoustic (FA) phonon branch.

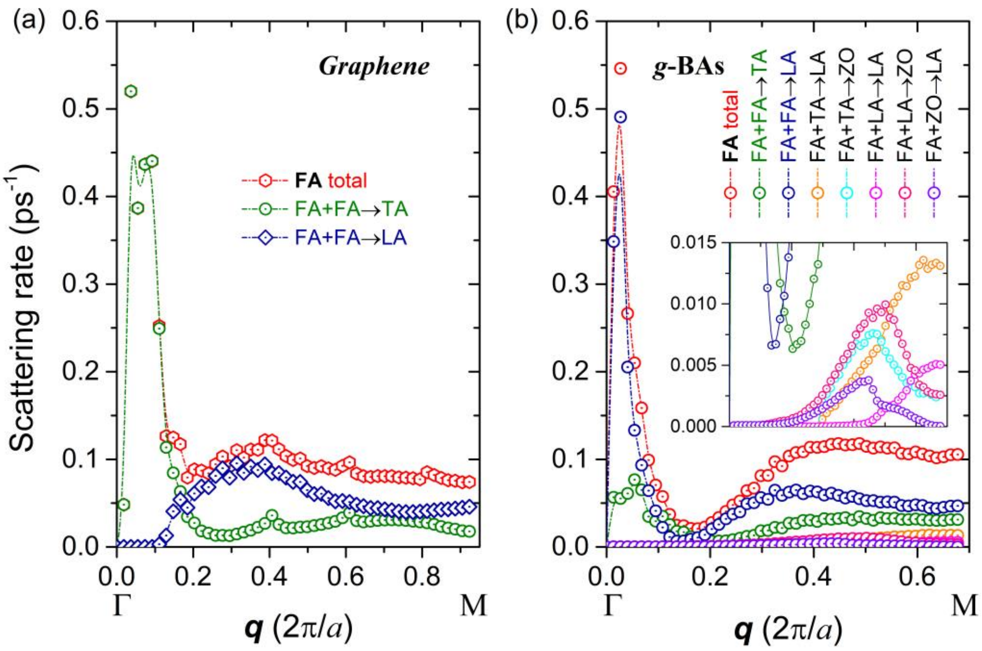


**Supplemental Figure 2.** The phonon–phonon scattering channels of the FA phonon branch along the Γ-M direction for (a) graphene and (b) *g*-BAs. The primary scattering channels are highlighted. Some other scattering channels are also plotted for reference, especially for *g*-BAs.

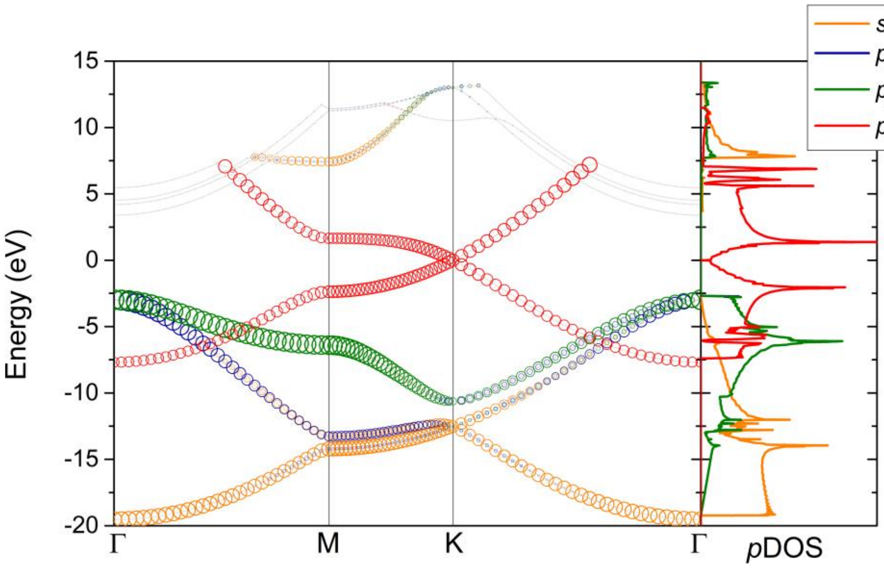


**Supplemental Figure 3.** The orbitals projected electronic band structures and density of states (DOS) for graphene.

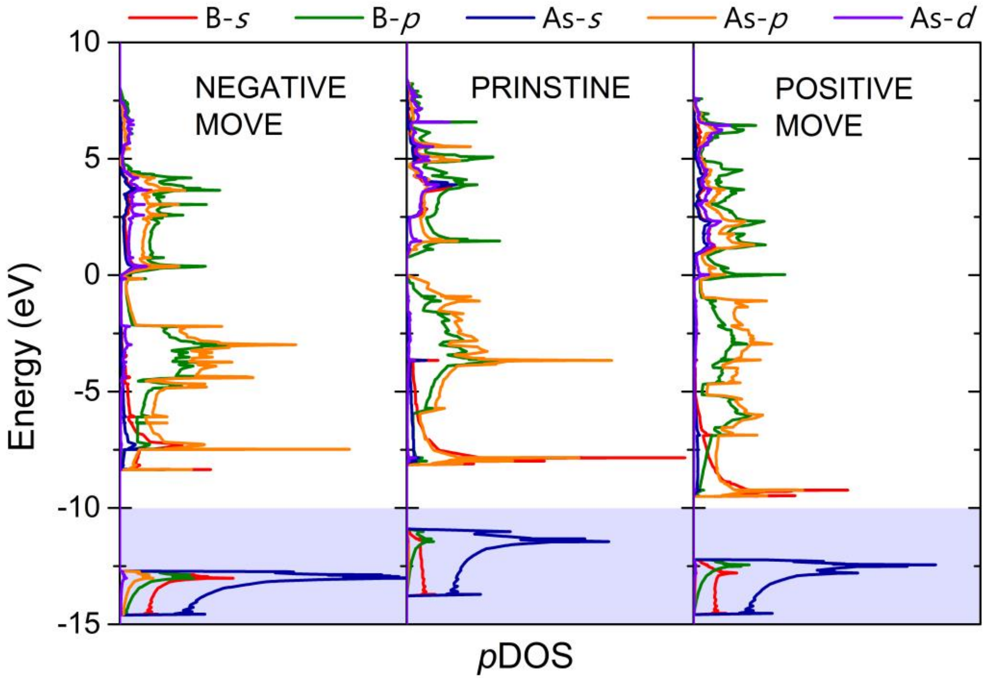


**Supplemental Figure 4.** The orbital projected electronic density of states (*p*DOS) of pristine g-BAs and the asymmetric response of *p*DOS to the displacement of As atom. The lone-pair As-*s* electrons are highlighted by the shaded area. The positive and negative moves mean the atomic displacement directions are opposite.

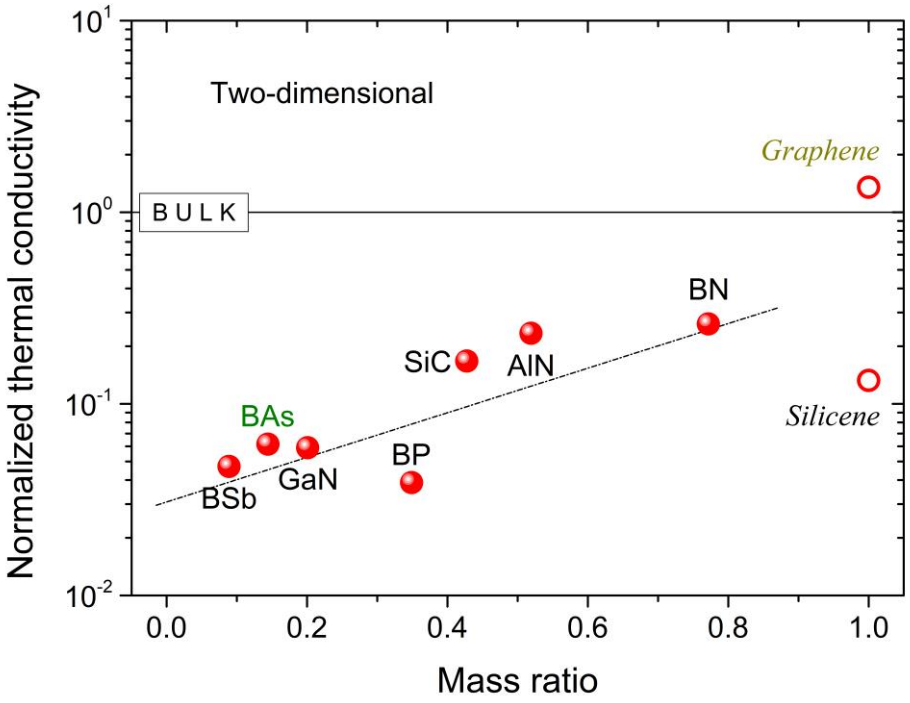


**Supplemental Figure 5.** The thermal conductivity of typical two-dimensional materials (graphene, silicene, BN, AlN, GaN, BP, BAs, BSb, and SiC) at 300 K, which are normalized to the bulk counterparts, respectively. The two-dimensional materials possess lower thermal conductivity compared to the bulk counterparts, except graphene. The dot line is for an eye guide. The specific data can be found in Supplemental Table 1.

## Supplemental Note 1: *Phonon-phonon scattering channels*

The phonon-phonon scattering channels ruled by the conservation of energy and momentum [**Eq. (2)** in the main text] quantify the specific scattering processes among different phonon branches, which can provide fundamental insight into the phonon scattering process [*Nanoscale* **8,** 11306-11319 (2016)]. Since the phonon branches are commonly degenerated or cross each other in most segments of the paths passing through the high-symmetry k-points in the BZ [**Figure 3(a)** in the main text], we only present the detailed scattering process of each phonon branch along the Γ-M direction, where phonon modes can be easily separated into different branches and the crossover problem is fixed manually (mainly for graphene). Note that the crossover between LA and ZO in g-BAs is not fixed due to too close frequency of the two branches (**Supplemental Figure 1**). The scattering rate for emission processes are multiplied by 1/2 to avoid counting twice for the same process.

First of all, we take graphene as an example to illustrate the symmetry-based selection rule of phonon–phonon scattering as proposed by Lindsay *et al.* [*Phys. Rev. B.* **82,** 115427 (2010)] based on the examination of potential energy under the symmetry operation. Because of the reflectional symmetry of the planar honeycomb structure, the phonon scattering processes involving odd numbers of FA modes are largely suppressed. As shown in the **Supplemental Figure 2(a)**, there are only two scattering channels in graphene: FA+FA→TA and FA+FA→LA. Although there are still other possible channels for the scattering of FA considering the conservation of energy and

momentum, they are all forbidden by the symmetry-based selection rule.

The situation is almost the same for *g*-BAs where the two primary scattering channels still hold. However, there exist also narrow scattering channels involving odd numbers of FA phonon modes of FA+TA/LA→LA/ZO [**Supplemental Figure 2(b)**]. The reason may lie in the fact that there exists strong coupling between LA and ZO in *g*-BAs due to the too close frequency of the two branches (**Supplemental Figure 1**). Thus, the scattering channels involving odd numbers of FA phonon modes are formed, leading to more scattering probability. Moreover, a close look at the planar honeycomb structure of g-BAs shows that due to the large difference in atomic radius and mass between B and As atoms, the planar honeycomb structure of *g*-BAs is not as perfectly smooth as that of graphene, leading to a lower symmetry group of *g*-BAs ($P\bar{6}M2$) than that of graphene (P6/MMM). The lower symmetry of *g*-BAs leads to the extra scattering channels by slightly breaking the symmetry based phonon–phonon scattering selection rule. Consequently, the contribution to thermal conductivity from FA is relatively smaller in *g*-BAs (26.9%) compared to graphene (85%).

## Supplemental Note 2: *More information on computational methods*

The force constant $C_{i\alpha;j\beta}$ can be obtained from the force caused by displacement [*Phys. Rev. B* **78,** 134106 (2008)]:

$$C_{i\alpha;j\beta} = -\frac{F_{i\alpha}}{\Delta_{j\beta}} ,$$

where $F_{i\alpha}$ is the force along the $\alpha$ direction acting on atom $i$ resulted from the displacement along the $\beta$ direction of atom $j$ ($\Delta_{j\beta}$). The amplitude of atomic displacement along the $\pm x$, $\pm y$, and $\pm z$ directions are 0.01 Å. The space group symmetry properties are used to reduce the calculation cost and numerical noise of the force constants, and it can also greatly simplify the determination of the dynamical matrix that is constructed based on the force constants [*Phys. Rev. B* **78,** 134106 (2008)]. The frequency and eigenvector forming the phonon dispersions can be obtained by diagonalizing the dynamical matrix

$$D = \frac{1}{\sqrt{m}} \sum_{\alpha;\beta} C_{i\alpha;j\beta} e^{iq(r_i - r_j)} .$$

The workflow and equations for calculating the thermal conductivity are described in the references related to the ShengBTE code [*Computer Physics Communications* **185,** 1747-1758 (2014); *Phys. Rev. B* **77,** 144112 (2008); *Phys. Rev. B* **86,** 174307 (2012)]. For example, the thermal conductivity could be obtained based on the equation:

$$\kappa_l^{\alpha\beta} = \frac{1}{k_B T^2 \Omega N} \sum_{\lambda} f_0(f_0 + 1)\,(\hbar\omega_\lambda)^2 v_\lambda^\alpha F_\lambda^\beta ,$$

where $\Omega$ is the volume of the unit cell, $f_0$ is the zero-order term of the phonon distribution function, $\lambda$ is the index of phonon mode comprising both phonon branch index and wave vector, $\omega$ is the angular frequency, $v$ is the group velocity, $F_\lambda$ is

defined based on the expansion of phonon distribution assuming the small enough $\nabla T$:

$$f_\lambda = f_0(\omega_\lambda) - F_\lambda \bullet \nabla T \frac{df_0}{dT},$$

and when only considering the scattering mechanism of two- and three-phonon process, $F_\lambda$ could be calculated with the formula:

$$F_\lambda = \tau_\lambda^0 (v_\lambda + \Delta_\lambda),$$

where $\tau_\lambda^0$ is the relaxation time obtained from perturbation theory:

$$\frac{1}{\tau_\lambda^0} = \frac{1}{N}\left(\sum_{\lambda'\lambda''}^{+} \Gamma^{+}_{\lambda\lambda'\lambda''} + \sum_{\lambda'\lambda''}^{-} \frac{1}{2}\Gamma^{-}_{\lambda\lambda'\lambda''} + \sum_{\lambda'} \Gamma_{\lambda\lambda'}\right),$$

where $\Gamma^{+}_{\lambda\lambda'\lambda''}$ and $\Gamma^{-}_{\lambda\lambda'\lambda''}$ are three-phonon scattering rates corresponding to absorption and emission processes of phonons, respectively, and $\Gamma_{\lambda\lambda'}$ is the scattering possibility from isotopic disorder. The full solution of BTE provides mode-dependent nonequilibrium populations to calculate the phonon-phonon scattering rates. The obtained lifetime can be interpreted based on the concept of relaxons (collective phonon excitations) [*Phys. Rev. X* **6,** 041013 (2016)], which are defined as the eigenstates of the scattering matrix and serve as the energy transport carriers.

The anharmonic nature of the system is quantified by the Grüneisen parameter, which can be calculated based on the change in phonon frequency with respect to the volume change ($\gamma = -\frac{V}{\omega}\frac{\partial \omega}{\partial V}$). The anharmonicity is described using the third order IFCs, while the contributions of the fourth and higher order terms are neglected. The third order (anharmonic) IFCs can be evaluated based on the third order derivatives of the

total energy with respect to the atomic displacement. The translational and rotational invariances of the third order IFCs are enforced using the Lagrange multiplier method [*Phys. Rev. B* **77,** 144112 (2008); *Phys. Rev. B* **86,** 174307 (2012)]. With the anharmonic IFCs, the scattering matrix can be constructed, based on which one can calculate all the three phonon scattering rates ($\Gamma^{+}_{\lambda\lambda'\lambda''}$ and $\Gamma^{-}_{\lambda\lambda'\lambda''}$) and then obtain the phonon lifetime. All the possible three-phonon scattering events, including the absorption and emission process, are determined based on the phonon dispersion by conserving both energy and crystal momentum. The dielectric tensor and Born effective charges are also obtained to take into account the long-range electrostatic interactions. The convergence test of thermal conductivity with respect to the cutoff distance and *Q*-grid are fully conducted, based on which the cutoff distance for the 3$^{rd}$ IFCs calculations is chosen larger than 6 Å.
